# Supplementary material for: PIFu: Pixel-Aligned Implicit Function for High-Resolution Clothed Human Digitization
Source: arXiv:1905.05172 source file (2019-12-03)
Supplement: Supplementary file 9 [file fig_results_video.tex]

\begin{figure*}[t]
\begin{center}
  \includegraphics[width=0.9\textwidth]{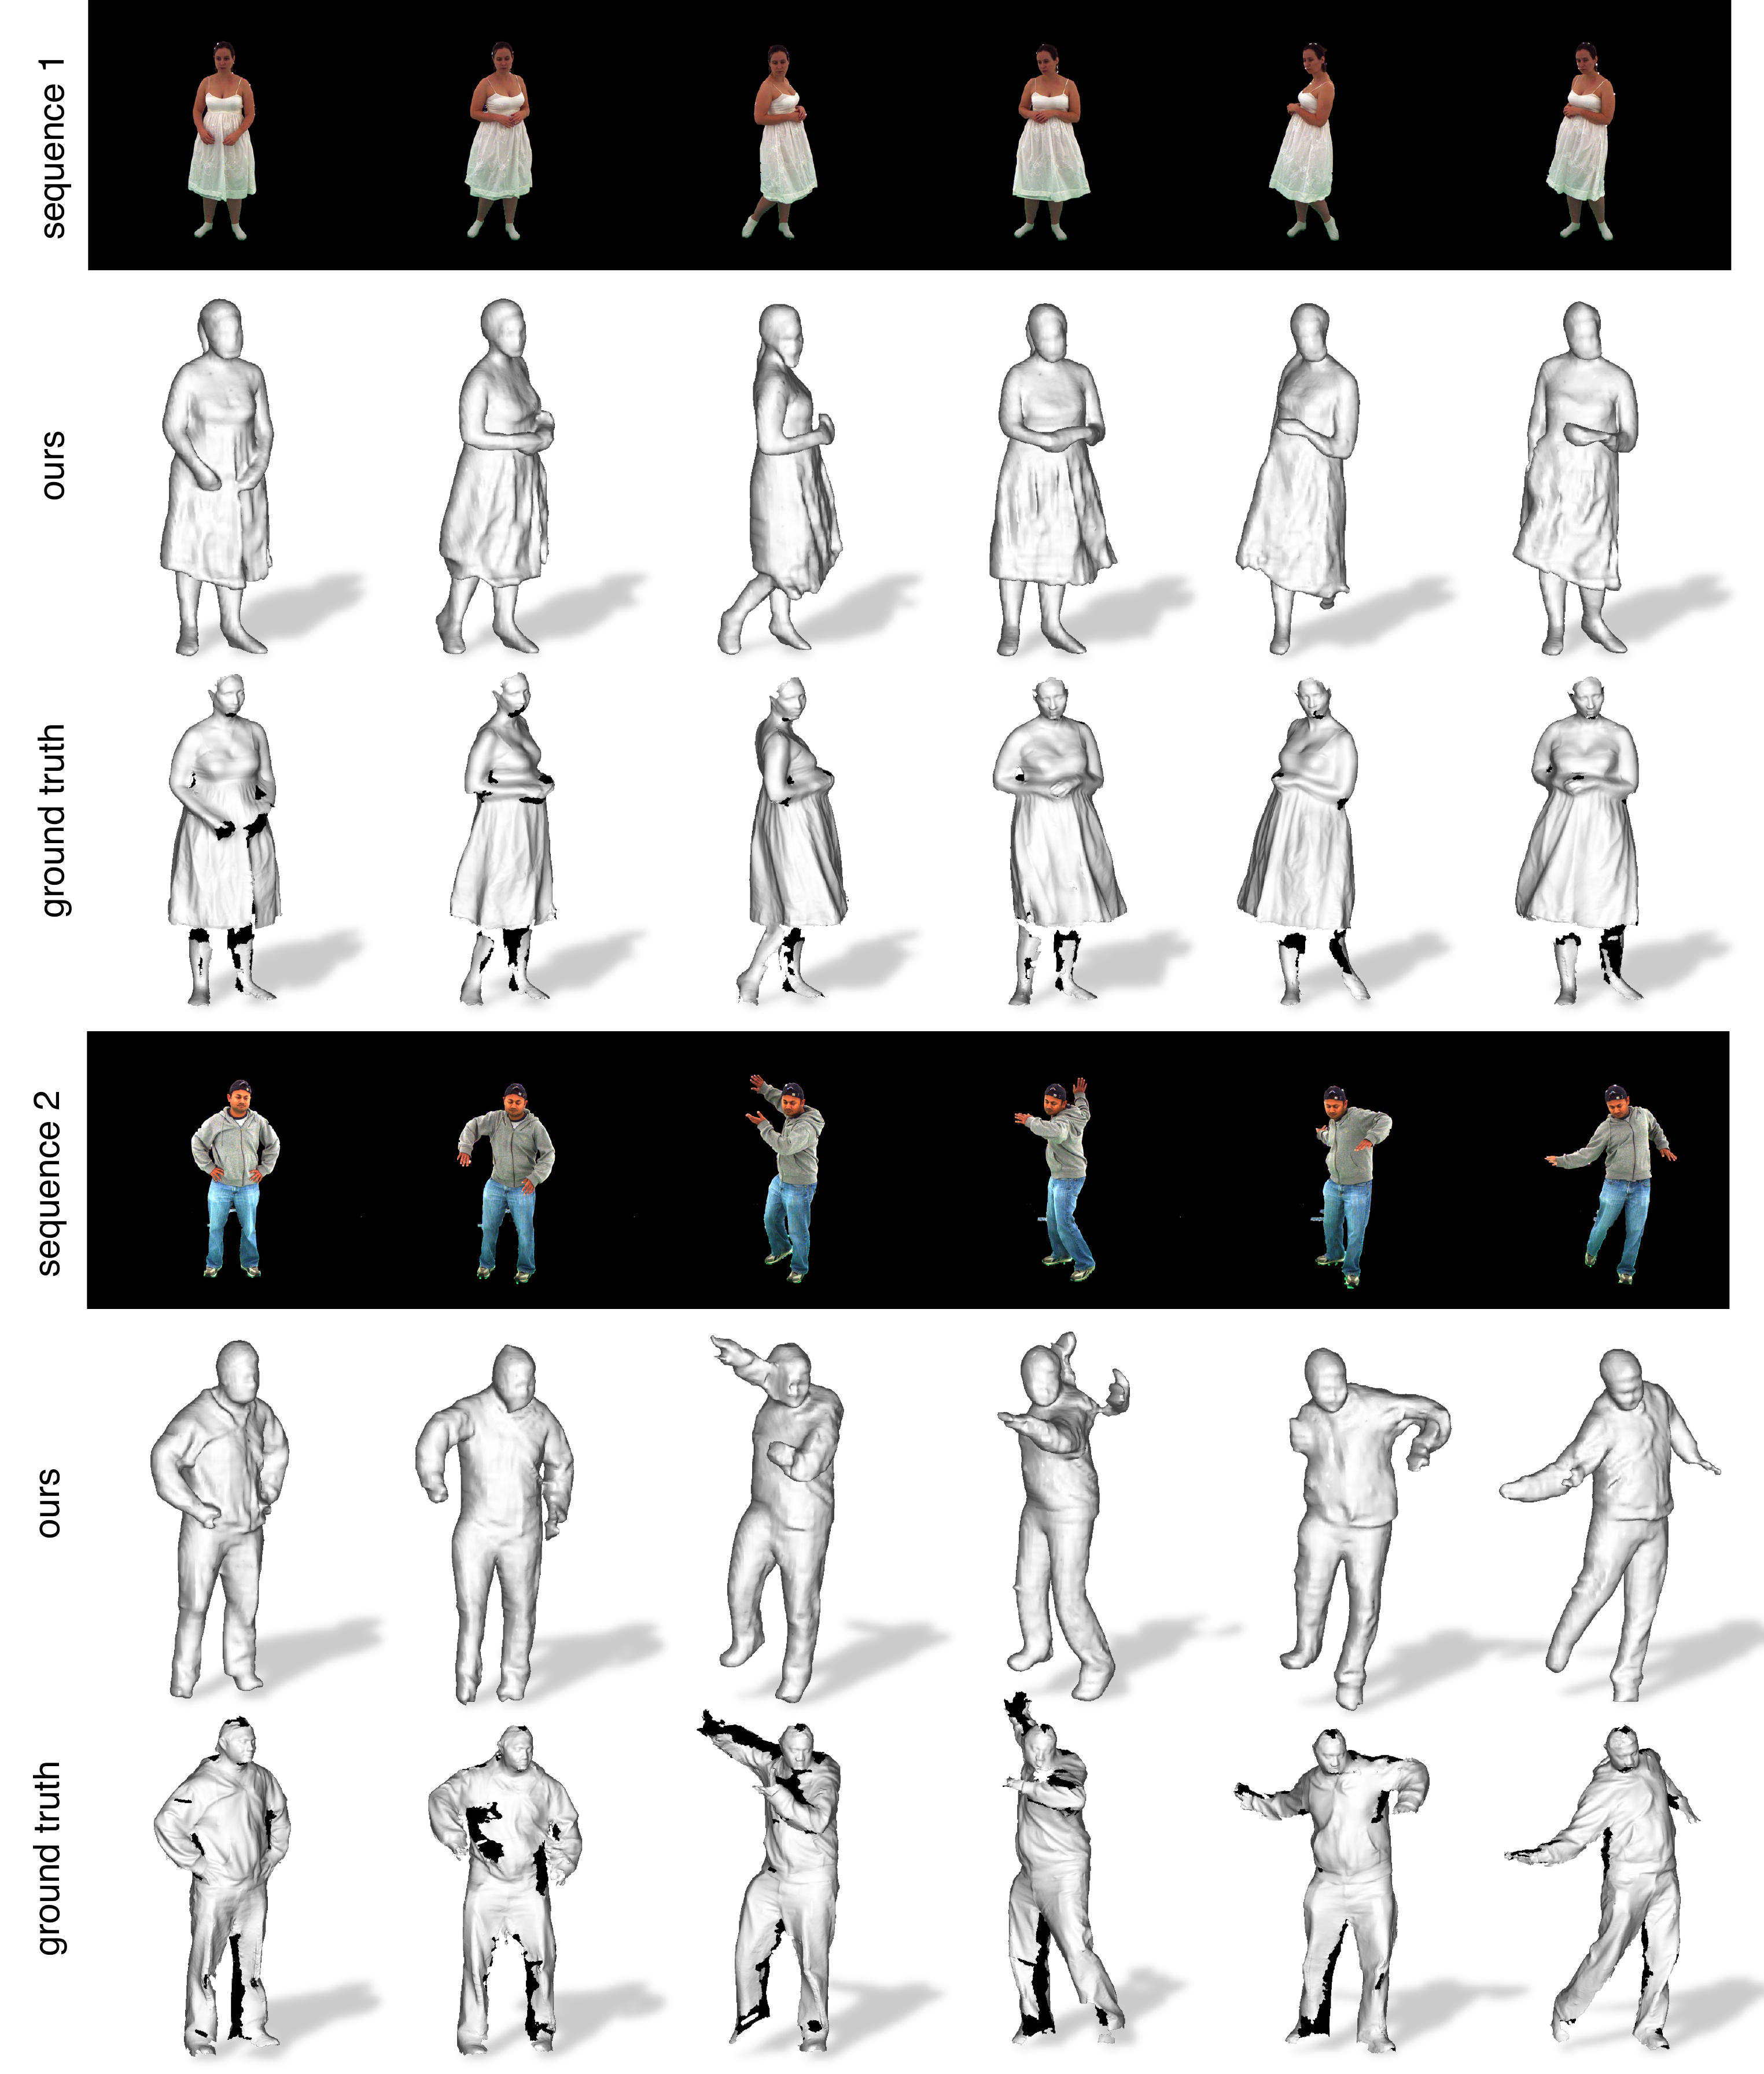}
\end{center}
\vspace{-10pt}
\caption{Results on video sequences obtained from \cite{vlasic2009dynamic}. While ours uses a single view input, the ground truth is obtained from $8$ views with controlled lighting conditions.}
\label{fig:video}
\end{figure*}
